# Supplementary material for: DROP: Dimensionality Reduction Optimization for Time Series
Source: arXiv:1708.00183 source file (2020-08-23)
Supplement: Supplementary file 1 [file appendices.tex]

\appendix
\section*{APPENDIX}

\section{Augmented Results}

In this section, we provide additional information to augment results provided in our time series case study. 
Table~\ref{tab:sample} displays the proportion of data required to attain a given $TLB$ when using a PCA transformation where output dimension is equal to input dimension. Table~\ref{tab:kneeded} illustrates the output dimension required for each algorithm (PAA, FFT, and PCA) to attain a target $TLB$. 
Table~\ref{tab:runtime-comparison} illustrates the different running times of each algorithm (PAA, FFT, and PCA), and how sampling using the proportion from Table~\ref{tab:sample} for $TLB=0.99$ can help bridge the time gap between SVD and other techniques. 
%Finally, we provide all of the remaining lesion studies for the UCR dataset.

\begin{table}[]
\centering
\caption{Normalized lower dimension for target $TLB$ across DR techniques. PCA admits lower dimension for most UCR time series datasets.}
\label{tab:kneeded}
\scriptsize
\begin{tabular}{|l|r|r|r|r|r|r|}
\hline
                                  & \multicolumn{3}{c|}{\textbf{TLB:0.75}}     & \multicolumn{3}{c|}{\textbf{TLB:0.99}}     \\ \hline
\textbf{Dataset (dimension)} & \textit{PAA} & \textit{FFT} & \textit{PCA} & \textit{PAA} & \textit{FFT} & \textit{PCA} \\ \hline
ElectricDevices (96)              & 0.126        & 0.094        & 0.032        & 0.594        & 0.212        & 0.164        \\ \hline
FordA (500)                       & 0.138        & 0.098        & 0.038        & 0.636        & 0.214        & 0.17         \\ \hline
FordB (500)                       & 0.018        & 0.029        & 0.009        & 0.290        & 0.177        & 0.035        \\ \hline
MALLAT (1024)                     & 0.084        & 0.068        & 0.057        & 0.898        & 0.837        & 0.522        \\ \hline
Phoneme (1024)                    & 0.004        & 0.026        & 0.001        & 0.049        & 0.035        & 0.034        \\ \hline
StarLightCurves (1024)            & 0.015        & 0.028        & 0.019        & 0.037        & 0.086        & 0.062        \\ \hline
UWGLAll (945)                     & 0.078        & 0.065        & 0.026        & 0.822        & 0.736        & 0.322        \\ \hline
wafer (152)                       & 0.014        & 0.030        & 0.007        & 0.103        & 0.049        & 0.037        \\ \hline
yoga (426)                        & 0.375        & 0.375        & 0.281        & 0.812        & 0.822        & 0.770        \\ \hline

\end{tabular}
\end{table}

\begin{table}[]
\centering
\caption{Runtime (in ms) of 3 DR techniques. PCA is slowest, and can be over $56\times$ slower than PAA. Running SVD over a sample can bridge this gap.}
\label{tab:runtime-comparison}
\scriptsize
\begin{tabular}{|l|c|c|c|c|}
\hline
\textbf{Dataset}        & \textbf{PAA ($\times$SVD)} & \textbf{FFT} & \textbf{SVD} & \textbf{Sampling} \\ \hline
ElectricDevices         & 3 (9.8$\times$)            & 18           & 33           & 6                 \\ \hline
FordA                   & 7 (19$\times$)             & 38           & 137          & 8                 \\ \hline
FordB                   & 7 (18$\times$)             & 32           & 121          & 7                 \\ \hline
MALLAT                  & 7 (37.6$\times$)           & 35           & 278          & 5                 \\ \hline
Phoneme                 & 5 (56.2$\times$)           & 29           & 281          & 164               \\ \hline
StarLightCurves         & 19 (24.1$\times$)          & 120          & 457          & 5                 \\ \hline
UWGLAll & 7 (43.5$\times$)           & 56           & 287          & 8                 \\ \hline
Wafer                   & 4 (6.1$\times$)            & 13           & 22           & 5                 \\ \hline
Yoga                    & 4 (21.2$\times$)           & 29           & 81           & 8                 \\ \hline
\end{tabular}
\end{table}

\begin{table}[]
\centering
\scriptsize
\caption{A small proportion of data is needed to obtain a $TLB$-preserving transform with full PCA (output = input dimension).}

\begin{tabular}{|l|r|r|r|}
\hline
                               & \multicolumn{3}{c|}{\textit{\textbf{TLB}}}    \\ \hline
\textbf{Dataset (number of datapoints)}               & \textbf{0.75} & \textbf{0.90} & \textbf{0.99} \\ \hline
ElectricDevices (16637)               & 0.0026        & 0.0043        & 0.0088        \\ \hline
FordA   (4921)                       & 0.0054        & 0.0114        & 0.0198        \\ \hline
FordB   (4446)                       & 0.008         & 0.0146        & 0.0248        \\ \hline
MALLAT  (2400)                       & 0.0031        & 0.009         & 0.0197        \\ \hline
Phoneme   (2110)                     & 0.0547        & 0.1346        & 0.3875        \\ \hline
StarLightCurves (9236)               & 0.001         & 0.0011        & 0.0039        \\ \hline
UWGLAll  (4478)       & 0.0025        & 0.0056        & 0.024         \\ \hline
wafer  (7164)                        & 0.001         & 0.0032        & 0.0097        \\ \hline
yoga  (3300)                         & 0.0017        & 0.0028        & 0.0096        \\ \hline
\end{tabular}
\label{tab:sample}
\end{table}
